# Supplementary material for: $^{27}$Al NMR spectroscopic and DFT computational study of the quadrupole coupling of aluminium in two polymorphs of the complex aluminium hydride CsAlH4
Source: arXiv:2410.07731 ancillary file (2024-10-10)
Supplement: Supplementary file 1 [file Poly_CsAlH4_Supp.pdf]

Supplementary Material:  
 $^{27}\text{Al}$  NMR spectroscopic and DFT computational  
study of the quadrupole coupling of aluminium in two  
polymorphs of the complex aluminium hydride  
 $\text{CsAlH}_4$

Bodo Zibrowius and Michael Fischer

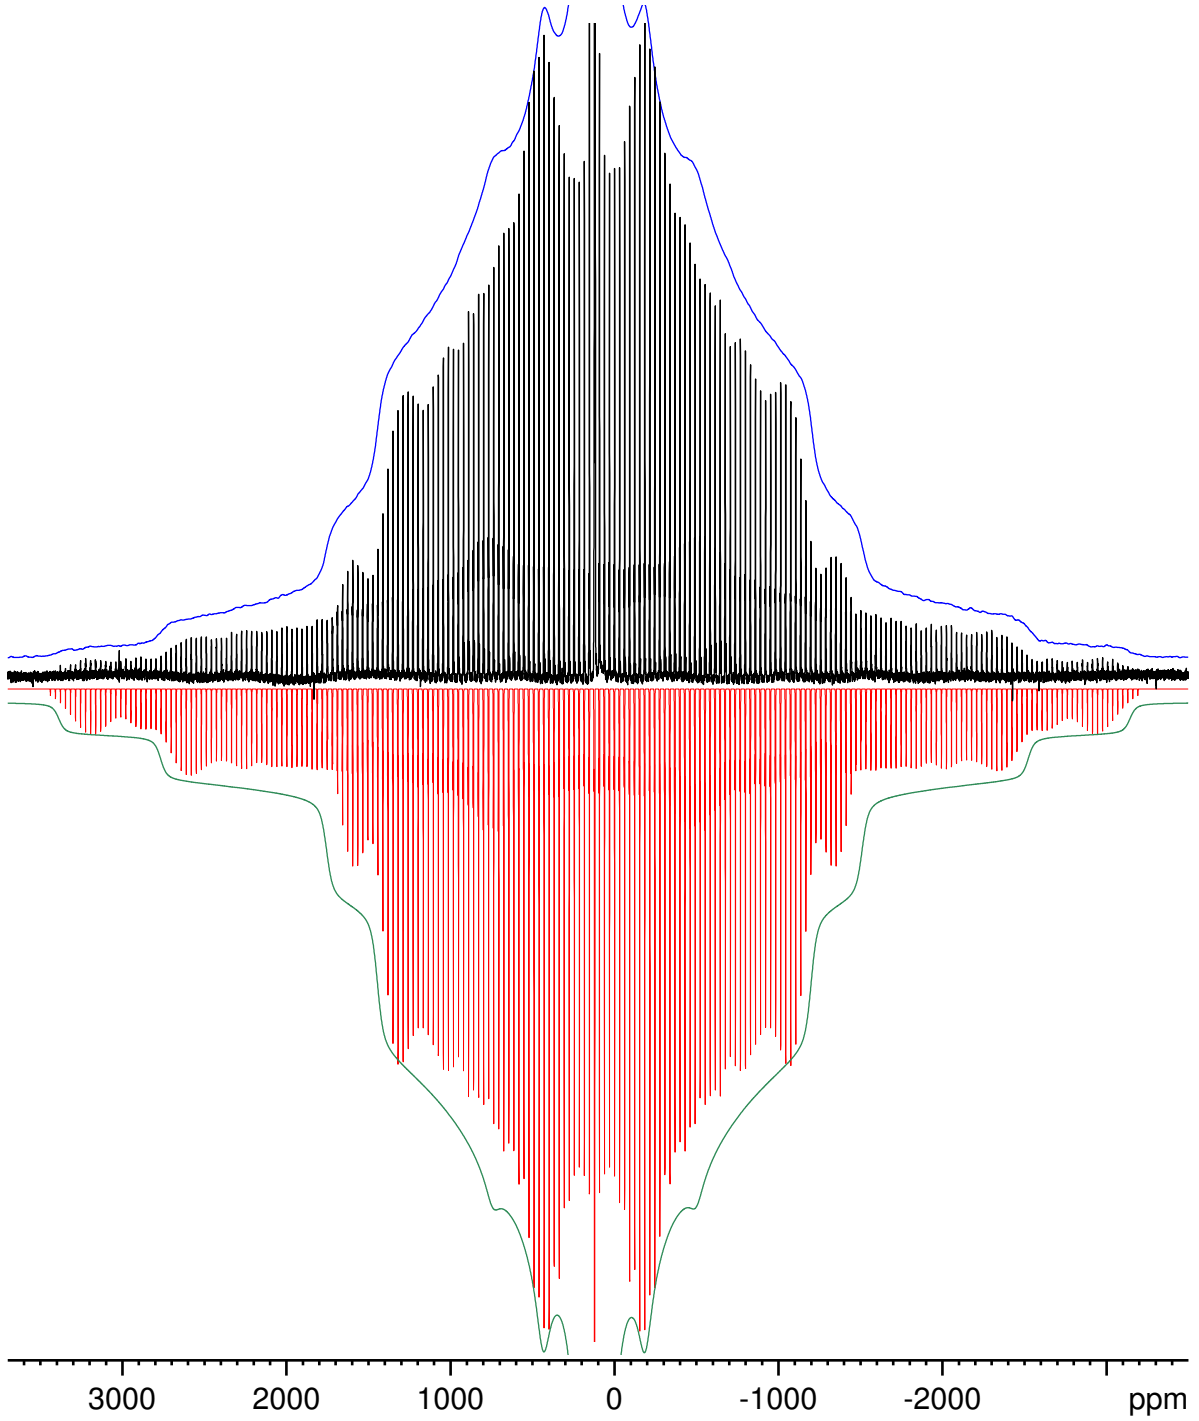

Figure S1: Experimental  $^{27}\text{Al}$  NMR spectra of  $\text{CsAlH}_4(o)$  measured for a stationary sample (blue) and the same sample spinning at  $\nu_{\text{MAS}} = 4$  kHz (black) and their simulations (green and red, respectively) with the parameters  $\delta_{\text{iso}} = 121.4$  ppm,  $C_Q = 1.42$  MHz and  $\eta = 0.62$ . To ease the comparison, the simulated spectra have been inverted. A Lorentzian line broadening with  $LB = 5000$  Hz and a Gaussian broadening with  $GB = 5000$  were used for the simulated static spectrum.

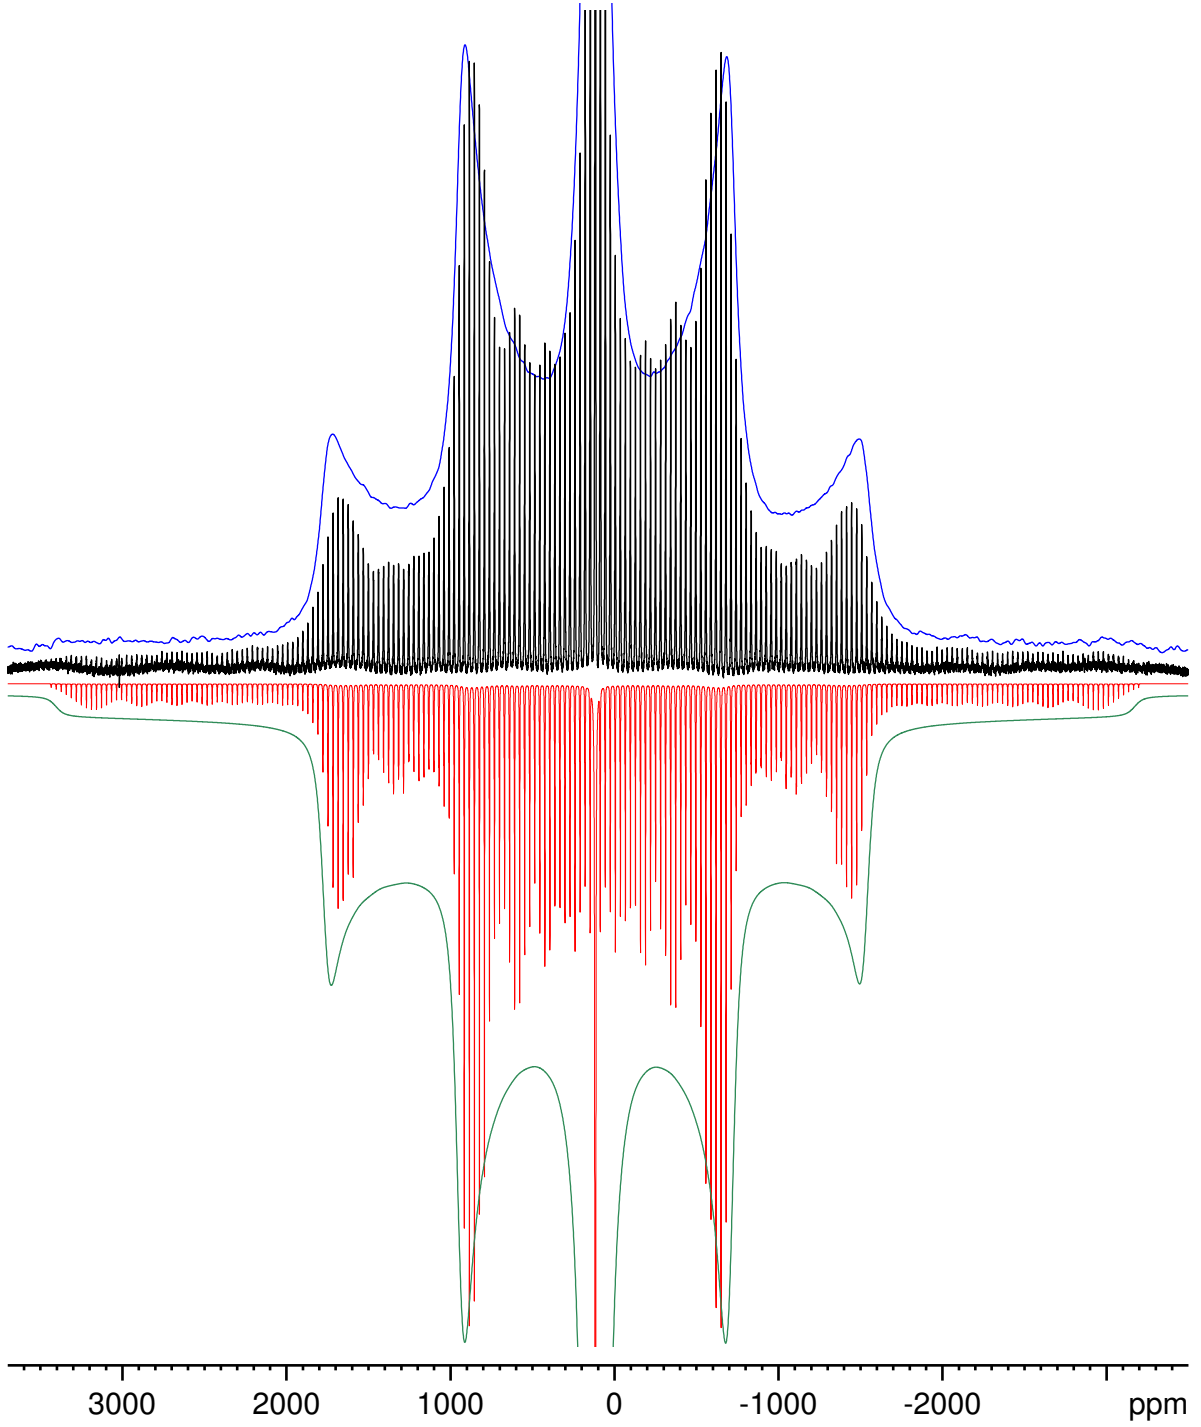

Figure S2: Experimental  $^{27}\text{Al}$  NMR spectra of  $\text{CsAlH}_4(t)$  measured for a stationary sample (blue) and the same sample spinning at  $\nu_{\text{MAS}} = 4 \text{ kHz}$  (black) and their simulations (green and red, respectively) with the parameters  $\delta_{\text{iso}} = 116.8 \text{ ppm}$ ,  $C_Q = 1.42 \text{ MHz}$  and  $\eta = 0$ . To ease the comparison, the simulated spectra have been inverted. A Lorentzian line broadening with  $LB = 8000 \text{ Hz}$  and a Gaussian broadening with  $GB = 5000$  were used for the simulated static spectrum.

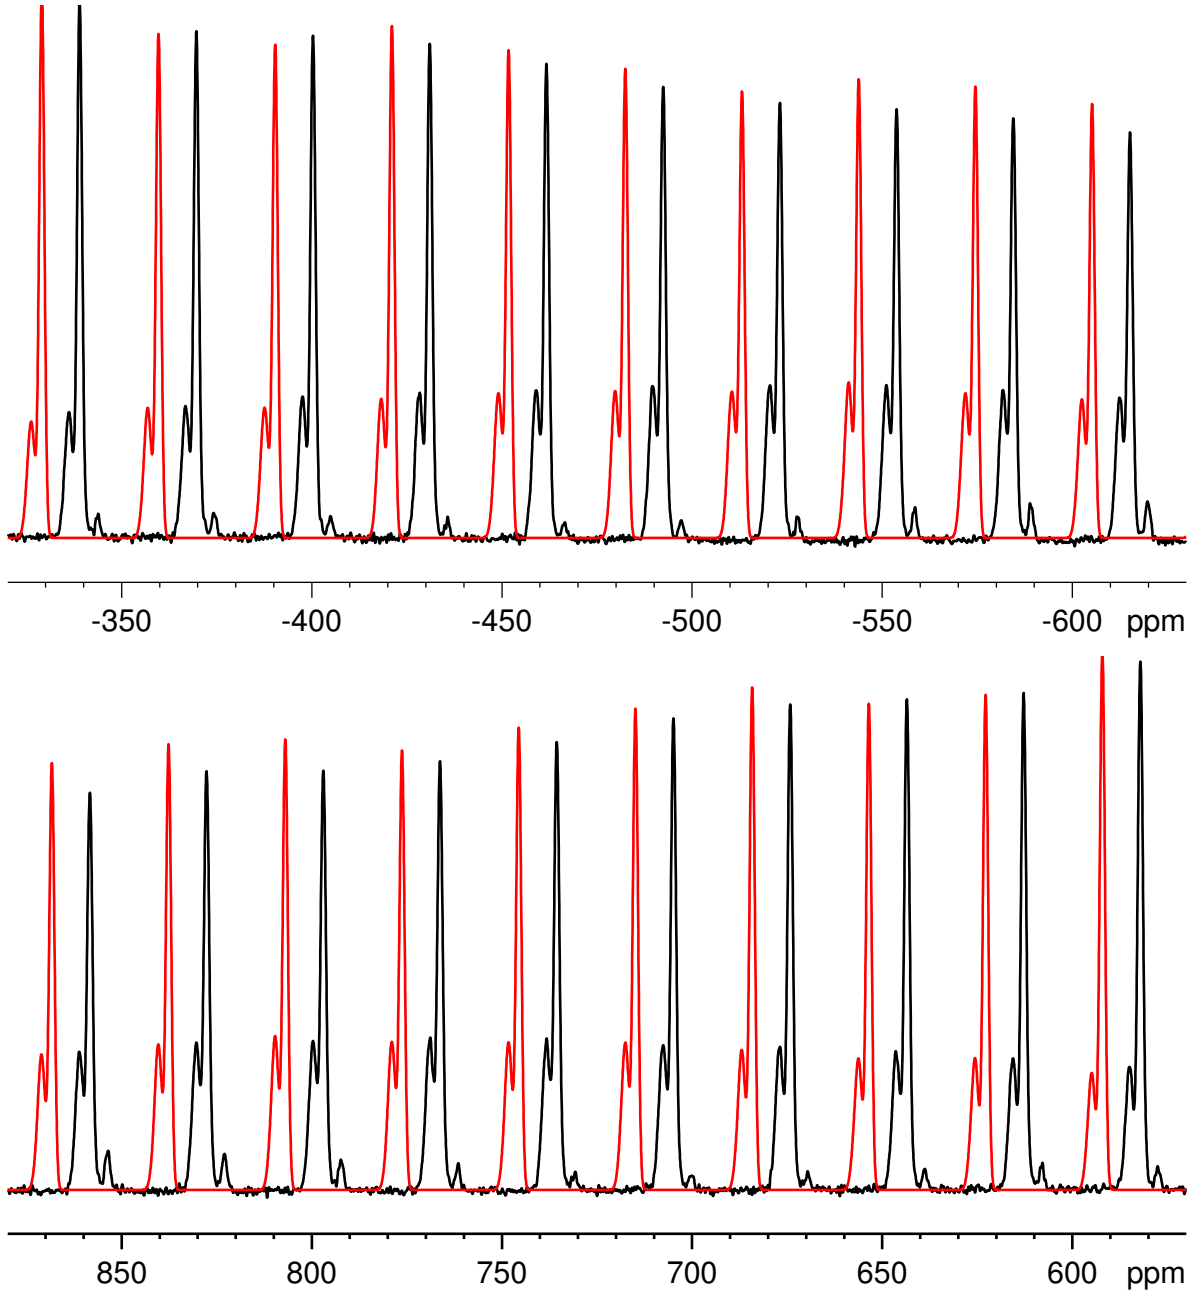

Figure S3: Experimental (black) and simulated (red)  $^{27}\text{Al}$  MAS NMR spectra of  $\text{CsAlH}_4(o)$  at  $\nu_{\text{MAS}} = 4\text{ kHz}$ . Only regions around the high-frequency (bottom) and low-frequency (top) maxima of the outer satellite transitions are shown. To ease the comparison, the simulated spectrum is given with an offset of +10 ppm with respect to the  $\delta$ -scale of the experimental one. The simulation with the parameters  $\delta_{\text{iso}} = 121.4\text{ ppm}$ ,  $C_Q = 1.42\text{ MHz}$  and  $\eta = 0.62$  nicely reproduces the sideband patterns of the satellite transitions. Since the simulation does not take into account the finite width of the pulses, the intensities of the sidebands in the outer wings of the spectrum are overestimated.

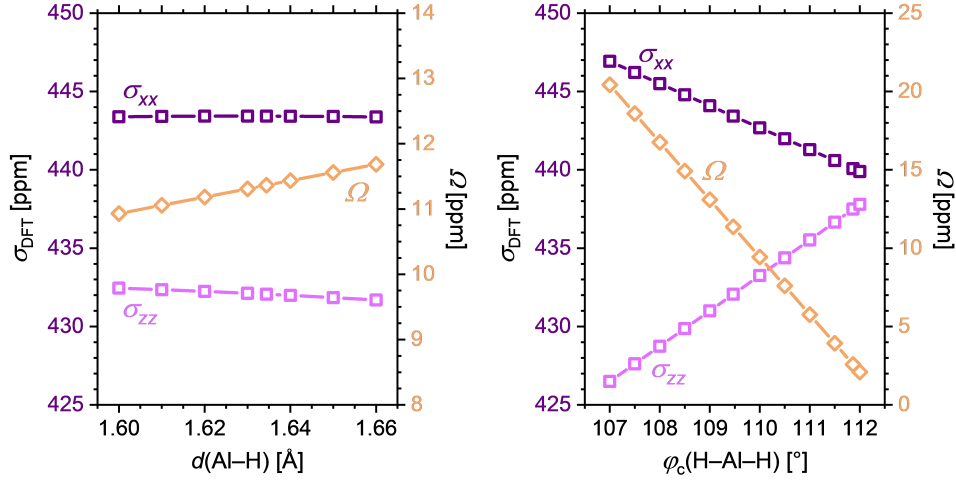

Figure S4: DFT-calculated chemical shielding parameters  $\sigma_{xx}$  and  $\sigma_{zz}$  and resulting span parameter  $\Omega = \sigma_{xx} - \sigma_{zz}$  obtained for  $\text{CsAlH}_4(t)$  structures with varied Al-H distances (left) and with varied H-Al-H angles (right).

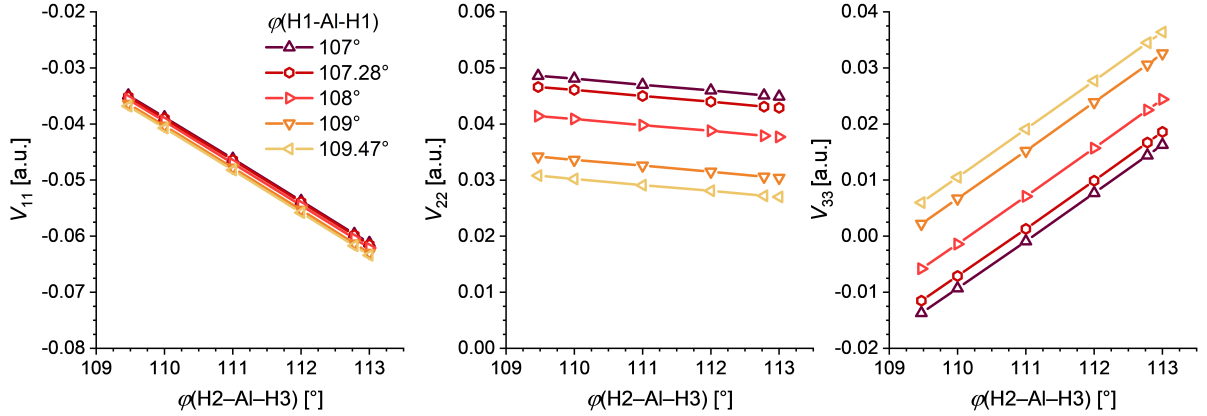

Figure S5: DFT-calculated eigenvalues of the EFG tensor obtained for  $\text{CsAlH}_4(o)$  structures with varied angles  $\phi(\text{H1-Al-H1})$  and  $\phi(\text{H2-Al-H3})$ . See list below Table S5 for information on the eigenvectors.

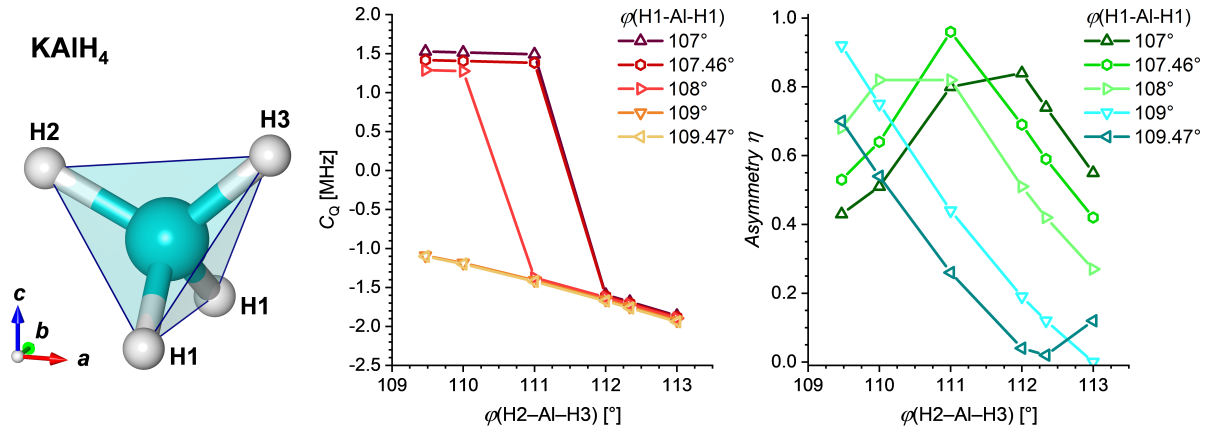

Figure S6: Left: Labelling of H atoms in  $\text{AlH}_4$  tetrahedron of  $\text{KAlH}_4$ . Center and right: DFT-GIPAW values of  $C_Q$  (center) and  $\eta$  (right) computed for  $\text{KAlH}_4$  structures in which the H-Al-H angles were varied.

Table S1: DFT-calculated NMR parameters obtained for  $\text{CsAlH}_4(t)$  structures with varied Al–H distances. All tetrahedral angles were set to  $109.47^\circ$ .

| $d(\text{Al-H})$ | $\sigma_{\text{iso}}$ | $\delta_{\text{iso}}$ | $\sigma_{xx}$ | $\sigma_{zz}$ | $\Omega$ | $C_Q$ |
|------------------|-----------------------|-----------------------|---------------|---------------|----------|-------|
| [Å]              | [ppm]                 | [ppm]                 | [ppm]         | [ppm]         | [ppm]    | [MHz] |
| 1.60             | 439.74                | 115.72                | 443.38        | 432.45        | 10.93    | 0.722 |
| 1.61             | 439.72                | 115.74                | 443.41        | 432.35        | 11.06    | 0.726 |
| 1.62             | 439.70                | 115.76                | 443.42        | 432.24        | 11.18    | 0.729 |
| 1.63             | 439.66                | 115.79                | 443.43        | 432.12        | 11.31    | 0.733 |
| 1.6344           | 439.64                | 115.81                | 443.42        | 432.06        | 11.36    | 0.734 |
| 1.64             | 439.61                | 115.84                | 443.42        | 431.99        | 11.43    | 0.736 |
| 1.65             | 439.55                | 115.89                | 443.40        | 431.84        | 11.56    | 0.739 |
| 1.66             | 439.48                | 115.96                | 443.38        | 431.69        | 11.69    | 0.741 |

Table S2: DFT-calculated NMR parameters obtained for  $\text{CsAlH}_4(t)$  structures with varied H–Al–H angles. The Al–H distance was fixed to the DFT-optimized value of 1.6344 Å.

| $\varphi_{\text{c}}(\text{H–Al–H})$ | $\sigma_{\text{iso}}$ | $\delta_{\text{iso}}$ | $\sigma_{xx}$ | $\sigma_{zz}$ | $\Omega$ | $C_{\text{Q}}$ |
|-------------------------------------|-----------------------|-----------------------|---------------|---------------|----------|----------------|
| [°]                                 | [ppm]                 | [ppm]                 | [ppm]         | [ppm]         | [ppm]    | [MHz]          |
| 107.0                               | 440.11                | 115.38                | 446.92        | 426.49        | 20.43    | -0.643         |
| 107.5                               | 440.01                | 115.47                | 446.21        | 427.62        | 18.59    | -0.367         |
| 108.0                               | 439.91                | 115.57                | 445.50        | 428.74        | 16.76    | -0.091         |
| 108.5                               | 439.82                | 115.65                | 444.79        | 429.87        | 14.92    | 0.188          |
| 109.0                               | 439.72                | 115.74                | 444.09        | 431.00        | 13.09    | 0.468          |
| 109.47                              | 439.64                | 115.81                | 443.42        | 432.06        | 11.36    | 0.734          |
| 110.0                               | 439.54                | 115.90                | 442.68        | 433.26        | 9.43     | 1.033          |
| 110.5                               | 439.45                | 115.98                | 441.99        | 434.39        | 7.60     | 1.318          |
| 111.0                               | 439.37                | 116.06                | 441.29        | 435.52        | 5.76     | 1.604          |
| 111.5                               | 439.28                | 116.14                | 440.59        | 436.66        | 3.93     | 1.892          |
| 111.86                              | 439.22                | 116.19                | 440.08        | 437.50        | 2.58     | 2.097          |
| 112.0                               | 439.19                | 116.22                | 439.89        | 437.80        | 2.09     | 2.180          |

Table S3: DFT-calculated  $\sigma_{\text{iso}}$  and  $\delta_{\text{iso}}$  values obtained for  $\text{CsAlH}_4(o)$  structures with varied angles  $\varphi(\text{H1-Al-H1})$  and  $\varphi(\text{H2-Al-H3})$ .

| $\varphi(\text{H1-Al-H1}) [^\circ] \rightarrow$ |                                     |        | 107    | 107.28 | 108    | 109    | 109.47 |
|-------------------------------------------------|-------------------------------------|--------|--------|--------|--------|--------|--------|
| $\sigma_{\text{iso}}$ [ppm]                     | $\varphi(\text{H2-Al-H3}) [^\circ]$ | 109.47 | 435.93 | 435.92 | 435.87 | 435.81 | 435.79 |
|                                                 | $\downarrow$                        | 110    | 435.91 | 435.89 | 435.84 | 435.78 | 435.76 |
|                                                 |                                     | 111    | 435.88 | 435.86 | 435.81 | 435.74 | 435.71 |
|                                                 |                                     | 112    | 435.87 | 435.85 | 435.79 | 435.72 | 435.68 |
|                                                 |                                     | 112.78 | 435.88 | 435.86 | 435.79 | 435.71 | 435.68 |
|                                                 |                                     | 113    | 435.89 | 435.86 | 435.8  | 435.71 | 435.68 |
| $\delta_{\text{iso}}$ [ppm]                     | $\varphi(\text{H2-Al-H3}) [^\circ]$ | 109.47 | 119.17 | 119.18 | 119.23 | 119.28 | 119.30 |
|                                                 | $\downarrow$                        | 110    | 119.19 | 119.21 | 119.25 | 119.31 | 119.33 |
|                                                 |                                     | 111    | 119.22 | 119.24 | 119.28 | 119.35 | 119.37 |
|                                                 |                                     | 112    | 119.23 | 119.25 | 119.30 | 119.36 | 119.40 |
|                                                 |                                     | 112.78 | 119.22 | 119.24 | 119.30 | 119.37 | 119.40 |
|                                                 |                                     | 113    | 119.21 | 119.24 | 119.29 | 119.37 | 119.40 |

Table S4: DFT-calculated  $\sigma_{ii}$  and resulting  $\Omega$  values obtained for  $\text{CsAlH}_4(o)$  structures with varied angles  $\varphi(\text{H1-Al-H1})$  and  $\varphi(\text{H2-Al-H3})$ .

| $\varphi(\text{H1-Al-H1}) [^\circ] \rightarrow$ |                                     |        | 107    | 107.28 | 108    | 109    | 109.47 |
|-------------------------------------------------|-------------------------------------|--------|--------|--------|--------|--------|--------|
| $\sigma_{xx}$ [ppm]                             | $\varphi(\text{H2-Al-H3}) [^\circ]$ | 109.47 | 441.76 | 441.70 | 441.53 | 441.28 | 441.16 |
|                                                 | $\downarrow$                        | 110    | 441.08 | 441.01 | 440.84 | 440.59 | 440.46 |
|                                                 |                                     | 111    | 439.83 | 439.76 | 439.59 | 439.32 | 439.19 |
|                                                 |                                     | 112    | 438.64 | 438.57 | 438.39 | 438.12 | 437.98 |
|                                                 |                                     | 112.78 | 437.76 | 437.69 | 437.50 | 437.45 | 437.75 |
|                                                 |                                     | 113    | 437.52 | 437.45 | 437.26 | 437.60 | 437.93 |
| $\sigma_{yy}$ [ppm]                             | $\varphi(\text{H2-Al-H3}) [^\circ]$ | 109.47 | 437.19 | 437.00 | 436.56 | 436.19 | 436.13 |
|                                                 | $\downarrow$                        | 110    | 437.19 | 437.00 | 436.59 | 436.29 | 436.28 |
|                                                 |                                     | 111    | 437.18 | 437.01 | 436.68 | 436.57 | 436.66 |
|                                                 |                                     | 112    | 437.18 | 437.05 | 436.85 | 436.99 | 437.20 |
|                                                 |                                     | 112.78 | 437.22 | 437.12 | 437.08 | 437.22 | 437.08 |
|                                                 |                                     | 113    | 437.24 | 437.16 | 437.16 | 436.97 | 436.83 |
| $\sigma_{zz}$ [ppm]                             | $\varphi(\text{H2-Al-H3}) [^\circ]$ | 109.47 | 428.85 | 429.05 | 429.52 | 429.97 | 430.08 |
|                                                 | $\downarrow$                        | 110    | 429.47 | 429.66 | 430.10 | 430.47 | 430.53 |
|                                                 |                                     | 111    | 430.64 | 430.81 | 431.16 | 431.33 | 431.28 |
|                                                 |                                     | 112    | 431.80 | 431.93 | 432.14 | 432.04 | 431.86 |
|                                                 |                                     | 112.78 | 432.66 | 432.75 | 432.80 | 432.47 | 432.19 |
|                                                 |                                     | 113    | 432.90 | 432.97 | 432.97 | 432.56 | 432.26 |
| $\Omega$ [ppm]                                  | $\varphi(\text{H2-Al-H3}) [^\circ]$ | 109.47 | 12.91  | 12.65  | 12.02  | 11.31  | 11.08  |
|                                                 | $\downarrow$                        | 110    | 11.61  | 11.35  | 10.75  | 10.12  | 9.93   |
|                                                 |                                     | 111    | 9.19   | 8.95   | 8.43   | 7.99   | 7.91   |
|                                                 |                                     | 112    | 6.85   | 6.65   | 6.26   | 6.07   | 6.12   |
|                                                 |                                     | 112.78 | 5.10   | 4.94   | 4.70   | 4.98   | 5.56   |
|                                                 |                                     | 113    | 4.62   | 4.48   | 4.29   | 5.04   | 5.67   |

Table S5: DFT-calculated eigenvalues  $V_{ii}$  and resulting quadrupole coupling constants  $C_Q$  and asymmetry parameters  $\eta$  obtained for  $\text{CsAlH}_4(o)$  structures with varied angles  $\varphi(\text{H1-Al-H1})$  and  $\varphi(\text{H2-Al-H3})$ .

|                 | $\varphi(\text{H1-Al-H1})$ [°] | →      | 107     | 107.28  | 108     | 109     | 109.47  |
|-----------------|--------------------------------|--------|---------|---------|---------|---------|---------|
| $V_{11}$ [a.u.] | $\varphi(\text{H2-Al-H3})$ [°] | 109.47 | -0.0349 | -0.0351 | -0.0356 | -0.0364 | -0.0368 |
|                 | ↓                              | 110    | -0.0388 | -0.0390 | -0.0395 | -0.0403 | -0.0407 |
|                 |                                | 111    | -0.0462 | -0.0464 | -0.0470 | -0.0478 | -0.0482 |
|                 |                                | 112    | -0.0537 | -0.0539 | -0.0545 | -0.0553 | -0.0558 |
|                 |                                | 112.78 | -0.0596 | -0.0598 | -0.0604 | -0.0613 | -0.0617 |
|                 |                                | 113    | -0.0612 | -0.0615 | -0.0621 | -0.0630 | -0.0634 |
|                 |                                |        |         |         |         |         |         |
| $V_{22}$ [a.u.] | $\varphi(\text{H2-Al-H3})$ [°] | 109.47 | 0.0486  | 0.0466  | 0.0414  | 0.0342  | 0.0308  |
|                 | ↓                              | 110    | 0.0481  | 0.0461  | 0.0409  | 0.0336  | 0.0302  |
|                 |                                | 111    | 0.0470  | 0.0450  | 0.0398  | 0.0326  | 0.0291  |
|                 |                                | 112    | 0.0460  | 0.0440  | 0.0388  | 0.0315  | 0.0281  |
|                 |                                | 112.78 | 0.0451  | 0.0431  | 0.0379  | 0.0306  | 0.0272  |
|                 |                                | 113    | 0.0449  | 0.0429  | 0.0377  | 0.0304  | 0.0270  |
|                 |                                |        |         |         |         |         |         |
| $V_{33}$ [a.u.] | $\varphi(\text{H2-Al-H3})$ [°] | 109.47 | -0.0137 | -0.0115 | -0.0058 | 0.0022  | 0.0060  |
|                 | ↓                              | 110    | -0.0093 | -0.0071 | -0.0014 | 0.0067  | 0.0105  |
|                 |                                | 111    | -0.0009 | 0.0013  | 0.0071  | 0.0152  | 0.0191  |
|                 |                                | 112    | 0.0077  | 0.0099  | 0.0157  | 0.0239  | 0.0277  |
|                 |                                | 112.78 | 0.0144  | 0.0167  | 0.0225  | 0.0306  | 0.0345  |
|                 |                                | 113    | 0.0163  | 0.0186  | 0.0244  | 0.0326  | 0.0364  |
|                 |                                |        |         |         |         |         |         |
| $C_Q$ [MHz]     | $\varphi(\text{H2-Al-H3})$ [°] | 109.47 | 1.675   | 1.606   | 1.428   | -1.253  | -1.267  |
|                 | ↓                              | 110    | 1.656   | 1.587   | 1.408   | -1.389  | -1.402  |
|                 |                                | 111    | 1.620   | -1.597  | -1.617  | -1.646  | -1.661  |
|                 |                                | 112    | -1.849  | -1.856  | -1.877  | -1.907  | -1.921  |
|                 |                                | 112.78 | -2.052  | -2.054  | -2.081  | -2.111  | -2.125  |
|                 |                                | 113    | -2.110  | -2.117  | -2.139  | -2.169  | -2.183  |
|                 |                                |        |         |         |         |         |         |
| $\eta$          | $\varphi(\text{H2-Al-H3})$ [°] | 109.47 | 0.44    | 0.51    | 0.72    | 0.88    | 0.67    |
|                 | ↓                              | 110    | 0.61    | 0.69    | 0.93    | 0.67    | 0.48    |
|                 |                                | 111    | 0.96    | 0.94    | 0.70    | 0.36    | 0.21    |
|                 |                                | 112    | 0.71    | 0.63    | 0.42    | 0.14    | 0.01    |
|                 |                                | 112.78 | 0.52    | 0.44    | 0.26    | 0.00    | 0.12    |
|                 |                                | 113    | 0.47    | 0.40    | 0.21    | 0.03    | 0.15    |
|                 |                                |        |         |         |         |         |         |

The eigenvalues  $V_{ii}$  are associated with the following eigenvectors:

- $V_{11}$ : Eigenvector  $[x, 0, z]$ , where  $0.99 \leq x \leq 1$  and  $-0.15 \leq z \leq 0$
- $V_{22}$ : Eigenvector  $[0, 1, 0]$
- $V_{33}$ : Eigenvector  $[x, 0, z]$ , where  $0 \leq x \leq 0.15$  and  $0.99 \leq z \leq 1$

Table S6: DFT-calculated  $\sigma_{\text{iso}}$ ,  $\delta_{\text{iso}}$ ,  $C_Q$ , and  $\eta$  values obtained for  $\text{KAlH}_4(o)$  structures with varied angles  $\varphi(\text{H1-Al-H1})$  and  $\varphi(\text{H2-Al-H3})$ .

| $\varphi(\text{H1-Al-H1}) [^\circ] \rightarrow$ |                                     |         | 107    | 107.46 | 108    | 109    | 109.47 |
|-------------------------------------------------|-------------------------------------|---------|--------|--------|--------|--------|--------|
| $\sigma_{\text{iso}}$ [ppm]                     | $\varphi(\text{H2-Al-H3}) [^\circ]$ | 109.47  | 448.41 | 448.37 | 448.32 | 448.24 | 448.21 |
|                                                 | $\downarrow$                        | 110     | 448.41 | 448.37 | 448.32 | 448.24 | 448.2  |
|                                                 |                                     | 111     | 448.43 | 448.38 | 448.33 | 448.24 | 448.2  |
|                                                 |                                     | 112     | 448.47 | 448.42 | 448.36 | 448.26 | 448.22 |
|                                                 |                                     | 112.34  | 448.48 | 448.43 | 448.37 | 448.27 | 448.22 |
|                                                 |                                     | 113     | 448.52 | 448.46 | 448.4  | 448.29 | 448.25 |
| $\delta_{\text{iso}}$ [ppm]                     | $\varphi(\text{H2-Al-H3}) [^\circ]$ | 109.47  | 107.86 | 107.90 | 107.94 | 108.02 | 108.04 |
|                                                 | $\downarrow$                        | 110     | 107.86 | 107.90 | 107.94 | 108.02 | 108.05 |
|                                                 |                                     | 111     | 107.84 | 107.89 | 107.93 | 108.02 | 108.05 |
|                                                 |                                     | 112     | 107.81 | 107.85 | 107.91 | 108.00 | 108.03 |
|                                                 |                                     | 112.34  | 107.80 | 107.84 | 107.90 | 107.99 | 108.03 |
|                                                 |                                     | 113     | 107.76 | 107.82 | 107.87 | 107.97 | 108.01 |
| $C_Q$ [MHz]                                     | $\varphi(\text{H2-Al-H3}) [^\circ]$ | 109.47  | 1.527  | 1.417  | 1.288  | -1.092 | -1.101 |
|                                                 | $\downarrow$                        | 110     | 1.515  | 1.405  | 1.276  | -1.186 | -1.199 |
|                                                 |                                     | 111     | 1.492  | 1.382  | -1.374 | -1.408 | -1.423 |
|                                                 |                                     | 112     | -1.594 | -1.608 | -1.626 | -1.658 | -1.674 |
|                                                 |                                     | 112.34  | -1.683 | -1.698 | -1.715 | -1.747 | -1.763 |
|                                                 |                                     | 113     | -1.863 | -1.877 | -1.893 | -1.924 | -1.939 |
| $\eta$                                          | $\varphi(\text{H2-Al-H3}) [^\circ]$ | 109.47  | 0.43   | 0.53   | 0.68   | 0.92   | 0.70   |
|                                                 | $\downarrow$                        | 110     | 0.51   | 0.64   | 0.82   | 0.75   | 0.54   |
|                                                 |                                     | 111     | 0.80   | 0.96   | 0.82   | 0.44   | 0.26   |
|                                                 |                                     | 112     | 0.84   | 0.69   | 0.51   | 0.19   | 0.04   |
|                                                 |                                     | 112.339 | 0.74   | 0.59   | 0.42   | 0.12   | 0.02   |
|                                                 |                                     | 113     | 0.55   | 0.42   | 0.27   | 0.00   | 0.12   |
